# Supplementary material for: Tunable strong coupling of mechanical resonance between spatially separated FePS$_3$ nanodrums
Source: arXiv:2107.01262 source file (2021-07-02)
Supplement: Supplementary file 1 [file Dumbells_SI.pdf]

# SUPPLEMENTARY INFORMATION: Tunable strong coupling of mechanical resonance between spatially separated $FePS_3$ nanodrums

Makars Šiškins,[*,†,‡] Ekaterina Sokolovskaya,[†,‡] Martin Lee,[‡] Samuel Mañas-Valero,[¶] Dejan Davidovikj,[‡] Herre S. J. van der Zant,[‡] and Peter G. Steeneken[*,‡,§]

†*These authors contributed equally.*

‡*Kavli Institute of Nanoscience, Delft University of Technology, Lorentzweg 1, 2628 CJ, Delft, The Netherlands*

¶*Instituto de Ciencia Molecular (ICMol), Universitat de València, c/Catedrático José Beltrán 2, 46980 Paterna, Spain*

§ *Department of Precision and Microsystems Engineering, Delft University of Technology, Mekelweg 2, 2628 CD, Delft, The Netherlands*

E-mail: m.siskins-1@tudelft.nl; p.g.steeneken@tudelft.nl

## 1. Continuum mechanics model of the circular membrane resonators of $FePS_3$

A flake, which is suspended over a circular cavity with a bottom gate electrode underneath, forms a capacitor-like structure. The mechanical response of the drum can be altered by applying a gate voltage. The change in the gate potential causes the flake to deflect, thereby

producing a shift in the resonance frequency. This method is used to tune the resonance frequency of the oscillators such that the frequency matching condition $\omega_1 = \omega_2$ and the avoided crossing are established.

Derivation of this section is closely following the one from Ref. 1. Due to the applied gate voltage, the membrane deflects with a mode shape, $\xi(a)$, under a uniformly distributed force:[2]

$$\xi(a) = x(1 - \frac{a^2}{r^2}), \tag{S1}$$

where $x$ is the deflection at the centre of the drum produced by the gate voltage, $r$ the radius of the drum and $a$ the radial distance from the centre of the drum. One can write the stored elastic energy due to the accumulated strain as:[3]

$$U_{\rm el} = \frac{\pi E h}{1-\nu^2}\int_0^a \left[\epsilon_0 + \frac{1}{2}\xi'^2(a)\right]^2 a\,{\rm d}a = \frac{\pi E h}{1-\nu^2}\left(\frac{2x^4}{3r^2} + \epsilon x^2 + \frac{1}{2}\epsilon^2 r^2\right), \tag{S2}$$

where $h$ is the thickness of the membrane, $E = 103$ GPa the Young's modulus and $\nu = 0.304$ Poisson's ratio of $FePS_3$,[4,5] $\epsilon$ and $\epsilon_0$ respectively the accumulated strain and the intrinsic pre-strain in the membrane, and $\xi'(a) = \frac{\partial \xi(a)}{\partial a}$.

For simplicity, the electrostatic energy, $U_{\rm es}$, of the capacitor formed by the suspended membrane and the gate electrode can be treated as:

$$U_{\rm es} = -\frac{1}{2}C_{\rm g}V_{\rm g}^2, \tag{S3}$$

where $C_{\rm g}$ is the gate capacitance and $V_{\rm g}$ the gate voltage. The capacitance increases as the sheet is deflected toward the gate electrode. We expand $C_{\rm g} \approx C_0 + x\frac{dC_{\rm g}}{dx} + \frac{x^2}{2}\frac{d^2C_{\rm g}}{dx^2}....$

Now, to find the equation of motion for the equilibrium position of the membrane centre due to electrostatic deflection at $x$, we set the total energy $U_{\rm el} + U_{\rm es}$ to a minimum:

$$U_{\rm el} + U_{\rm es} = \frac{8\pi E h}{3(1-\nu^2)r^2}x^3 + \left(\frac{2\pi E h \epsilon_0}{1-\nu^2} - \frac{1}{2}C''_{\rm g}V_{\rm g}^2\right)x - \frac{1}{2}C'_{\rm g}V_{\rm g}^2 = 0. \tag{S4}$$

Then, we find the spring constant $k$ of the membrane as:

$$k = \left.\frac{\partial^2 \left(U_{\mathrm{el}} + U_{\mathrm{es}}\right)}{\partial x^2}\right|_{x_{\mathrm{g}}} = \frac{2\pi E h \epsilon_0}{1-\nu^2} + \frac{8\pi E h}{\left(1-\nu^2\right) r^2} x_{\mathrm{g}}^2 - \frac{1}{2} C_{\mathrm{g}}'' V_{\mathrm{g}}^2, \tag{S5}$$

where $x_{\mathrm{g}}$ is the maximal deflection at the membrane centre and $C_{\mathrm{g}}'' = \frac{\partial^2 C_{\mathrm{g}}}{\partial x^2}$. The exact solution of eq S4 for $x_{\mathrm{g}}$ is rather complex.[1] However, following the approach in Ref. 6 one can approximate this value as:

$$x_{\mathrm{g}} \approx \frac{\varepsilon_0 r_{\mathrm{g}}^2}{8 x_{\mathrm{c}}^2 T} V_{\mathrm{g}}^2, \tag{S6}$$

where $x_{\mathrm{c}} = 220$ nm is the cavity gap size, $r_{\mathrm{g}} = 2.5$ $\mu$m the radius of the bottom gate electrode, and $T = Eh\frac{\epsilon}{1-\nu}$ the membrane tension.

Using eq. S5, we find the resonance frequency of the fundamental vibration mode of the drum, $\omega_0$, by including both membrane and plate contributions:[7]

$$\omega_0 \approx \sqrt{\omega_{\mathrm{membrane}}^2 + \omega_{\mathrm{plate}}^2} = \sqrt{\frac{k}{m_{1,2}} + \left(\frac{10.21 h}{2r^2}\right)^2 \frac{E}{3\rho(1-\nu^2)}}, \tag{S7}$$

where $m_{1,2}$ is the effective mass and $\rho = 3375$ kg/m$^3$ the mass density of $FePS_3$.

We use a combination of eq S5, S6 and S7 to model $\omega(V_{\mathrm{g}})$ of both drums. As shown in Figure S1, the model describes closely the experiment for both membranes. For drum 1, we used $\epsilon = 0.274\%$, which is within expected values[4] at $T = 4$ K, an effective mass of $m_1 = 620$ fg, which is close to the theoretical value of $m_{\mathrm{eff}} = 0.27\rho h \pi r^2 = 659.58$ fg, and $C_{\mathrm{g},1}'' = 2.66$ mF/m$^2$, which is slightly smaller than the estimate[6,8] $C_{\mathrm{g}}'' \approx \frac{0.542\varepsilon_0 \pi r_{\mathrm{g}}^2}{x_{\mathrm{c}}^3} = 8.85$ mF/m$^2$. For drum 2, we used $\epsilon = 0.279\%$, an effective mass of $m_2 = 624.6$ fg, and $C_{\mathrm{g},2}'' = 2.6$ mF/m$^2$.

# 2. Joule dissipation model

An applied gate voltage, $V_{\mathrm{g}}$, to the membrane can induce capacitive displacement currents due to the periodic change of capacitance induced by the mechanical motion.[8,9] These cur-

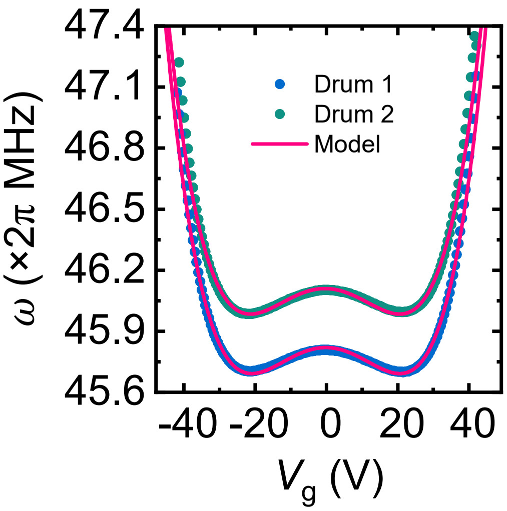


Figure S1: Frequency $\omega(V_g)$ of the resonance peaks for two drums (the same as in the main text Fig. 1.) at 4 K. Filled dots - measured data, Solid lines - continuum mechanics model of eq S5, S6 and S7.

rents consequently can decrease the quality factor via Joule dissipation.[8] We derive the equation for the Joule dissipation model for a circular membrane of $FePS_3$ closely following the approach from Ref. 8 and 9.

Membrane oscillations cause its periodic deflection and thus variations in the distance between the membrane and the gate electrode. This gives rise to a time-varying capacitance $C(t) = C_{eq} + \delta C \cos(\omega_d t)$, where $C_{eq}$ is the geometrical capacitance at equilibrium position of the membrane, $\delta C$ the capacitance oscillation amplitude, and $\omega_d$ the drive frequency of the membrane. The induced displacement currents, $I_d$, in the membrane generated by $V_g$ and time- varying capacitance $C(t)$ are described by $I_d(V_g) = \omega_d V_g \delta C \sin(\omega_d t)$. Assuming that the effective resistance of $FePS_3$ membranes $R_{1,2}$ does not change significantly with $V_g$, the energy dissipated per period by the displacement current $U_d$ is:

$$U_d(V_g) \approx R_{1,2} \int_0^{2\pi/\omega_d} I_d^2 dt = \pi R_{1,2}\, \omega_d\, (\delta C)^2\, V_g^2. \tag{S8}$$

The dissipation due to displacement currents is found as $\frac{1}{Q_d(V_g)} = \frac{U_d(V_g)}{2\pi U_t}$, where $U_t$ is the

total energy stored in the resonator. The total dissipation $\frac{1}{Q_{1,2}}$ is:

$$\frac{1}{Q_{1,2}} = \frac{1}{Q_0} + \frac{1}{Q_\mathrm{d}(V_\mathrm{g})} = \frac{1}{Q_0} + \frac{R_{1,2}\,\omega_\mathrm{d}}{2U_\mathrm{t}}\,(\delta C)^2\,V_\mathrm{g}^2. \tag{S9}$$

Considering the corresponding mechanical energy dissipation rates $\gamma_{1,2} = \frac{\omega_{1,2}}{Q_{1,2}}$ of $FePS_3$ membranes at a resonance frequency $\omega_d = \omega_{1,2}$, eq S9 can be rewritten in terms of $\gamma_{1,2}$:

$$\gamma_{1,2} = \frac{\omega_{1,2}}{Q_0} + \frac{\omega_{1,2}}{Q_\mathrm{d}(V_\mathrm{g})} = \gamma_0 + \frac{R_{1,2}\,\omega_{1,2}^2}{2U_\mathrm{t}}\,(\delta C)^2\,V_\mathrm{g}^2 = \gamma_0 + \frac{R_{1,2}}{m_{1,2}}\left(\frac{\partial C_\mathrm{g}}{\partial x}\right)^2 V_\mathrm{g}^2, \tag{S10}$$

where $\frac{\partial C_\mathrm{g}}{\partial x} \approx \frac{\varepsilon_0 \pi r_\mathrm{g}^2}{x_\mathrm{c}^2}$. We use $m_{1,2}$ for each resonator from SI 1 and plot the model of eq S10 versus the measured $\gamma_{1,2}$. As shown in Figure S2a, model describes the experiment well in case of drum 1 with $\gamma_0 = 11.76$ kHz and $R_1 = 721.4\ \Omega$. In Figure S2b, the model is also shown for drum 2 following the experiment closely with $\gamma_0 = 11.75$ kHz and $R_2 = 937.1\ \Omega$.

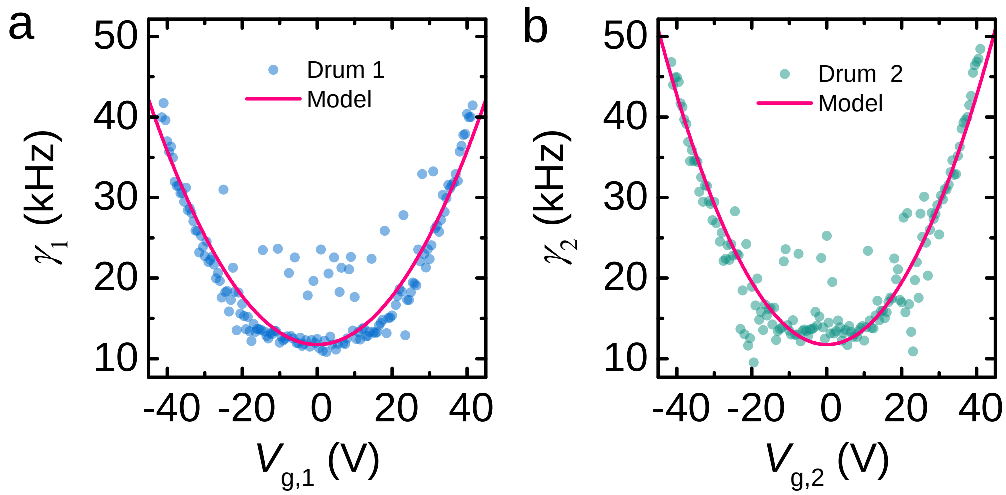


Figure S2: Dissipation rate $\gamma_{1,2}(V_\mathrm{g})$ of the resonance peaks for two drums (the same as in the main text Fig. 1.) at 4 K. (a,b) Filled dots - measured data, Solid lines - Joule dissipation model of eq S10.

## 3. Linear coupled oscillators model

In order to predict the measured response, we describe our system as a pair of damped resonators characterized with their effective masses $m_1$ and $m_2$ and corresponding positions $x_1(t)$, $x_2(t)$ (depicted in Figure S3). The derivation closely follows the one from Ref. 10. The coupling potential between the oscillators is defined in a bi-linear form $V_{int} = -Jx_1x_2$, where $J$ is the coupling parameter. In an experiment, multiple mechanisms can contribute to $J$, such that it is approximately equal to the sum of individual contributions:

$$J \approx J_{\text{mech}} + J_{\text{el}} + J_{\text{ph}} + J_{\text{other}}, \tag{S11}$$

where $J_{\text{mech}}$ is the direct mechanical contribution to coupling, $J_{\text{el}}$ the electrical coupling parameter, $J_{\text{ph}}$ is the coupling via a phonon bath in the material, and $J_{\text{other}}$ accounts for other possible mechanisms of coupling. In our case, the electrical coupling parameter $J_{\text{el}}$, that is related to the capacitive ground between the flake and the top electrode as will be described in SI 4, is $J_{\text{el}} \gg J_{\text{mech}}, J_{\text{ph}}, J_{\text{other}}$ and acts as the dominant coupling mechanism, so $J \approx J_{\text{el}}$.

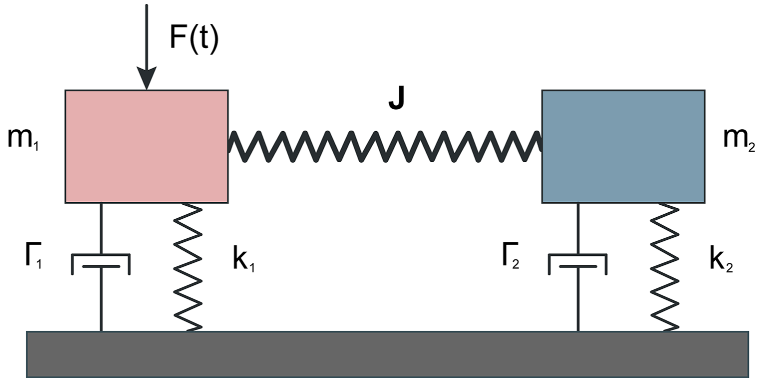


Figure S3: Schematic drawing of two linearly coupled damped resonators. $\Gamma_{1,2}$ is the damping parameter, $F(t)$ the driving force, $k_{1,2}$ the spring constant.

Let us assume that an external force of amplitude $F$ and drive frequency $\omega_{\text{d}}$ is applied

to one of the resonators resulting in motion that is described as:

$$\begin{cases} m_1\ddot{x_1} + \Gamma_1\dot{x_1} + k_1x_1 = Jx_2 + F\,\cos\omega_\text{d}t, \\ m_2\ddot{x_2} + \Gamma_2\dot{x_2} + k_2x_2 = Jx_1, \end{cases} \tag{S12}$$

where $\Gamma_{1,2}$ is the damping coefficient, $k_{1,2}$ the stiffness of the corresponding oscillator. The same equation can be presented in a different form:

$$\begin{cases} \ddot{x_1} + \gamma_1\dot{x_1} + \omega_1^2x_1 = \frac{J}{m_1}x_2 + f_\text{d}\,\cos\omega_\text{d}t, \\ \ddot{x_2} + \gamma_2\dot{x_2} + \omega_2^2x_2 = \frac{J}{m_2}x_1, \end{cases} \tag{S13}$$

where $\gamma_{1,2}$ is the dissipation ratio, $\omega_{1,2} = \sqrt{\frac{k_{1,2}}{m_{1,2}}}$ the natural frequency, and $f_\text{d} = F/m_1$ the re-scaled force. When two resonators are of a similar effective mass $m_1 \approx m_2$, the coupling coefficient $J$ can be expressed as $j = \frac{J}{\sqrt{m_1m_2}} \approx \frac{J}{m_{1,2}}$, which further simplifies the equation to:

$$\begin{cases} \ddot{x_1} + \gamma_1\dot{x_1} + \omega_1^2x_1 = jx_2 + f_\text{d}\,\cos\Omega t, \\ \ddot{x_2} + \gamma_2\dot{x_2} + \omega_2^2x_2 = jx_1. \end{cases} \tag{S14}$$

At some point in time, the system of eq S14 attains a steady-state motion with two resonators developing synchronized motion at a drive frequency $\omega_\text{d}$. This stationary state can be described by:

$$\begin{cases} x_1(t) = A_1\cos(\omega_\text{d}t + \phi_1) = \text{Re}[A_1\,e^{i(\omega_\text{d}t+\phi_1)}], \\ x_2(t) = A_2\cos(\omega_\text{d}t + \phi_2) = \text{Re}[A_2\,e^{i(\omega_\text{d}t+\phi_2)}]. \end{cases} \tag{S15}$$

We now introduce non-dimensional rescaled detuning $\delta_{1,2} = \frac{\omega_{1,2}^2-\omega_\text{d}^2}{\gamma_{1,2}\,\omega_\text{d}}$ which captures the difference between the driving frequency $\omega_\text{d}$ and natural frequencies $\omega_{1,2}$ of corresponding resonators. With this substitution, $x_{1,2}(t)$ is a solution[10] to eq S14 if amplitudes $A_{1,2}$ are

equal to:

$$\begin{cases} A_1 = \frac{f_\mathrm{d}}{\gamma_1\omega_\mathrm{d}}\frac{\sqrt{\delta_2^2+1}}{\triangle}, \\ A_2 = \frac{f_\mathrm{d}}{\gamma_1\gamma_2\omega_\mathrm{d}^2}\frac{|j|}{\triangle}, \end{cases} \tag{S16}$$

where $\triangle = \sqrt{(\Lambda+1-\delta_1\delta_2)^2+(\delta_1+\delta_2)^2}$, and $\Lambda = \frac{j^2}{\gamma_1\gamma_2\omega_\mathrm{d}^2}$ the coupling strength coefficient. Due to the symmetry between equations in eq S14, $A_1$ describes the amplitude of the driven resonator and $A_2$ the amplitude of the non-driven one. In Figure S4 we show an example of a fit of the measured data at 4 K, $V_{\mathrm{g},1} = 37.21$ V and $V_{\mathrm{g},2} = 30$ V to the model of eq S16. We use $\gamma_{1,2}(V_\mathrm{g})$ and $\omega_{1,2}(V_\mathrm{g})$ from the data in Fig. 1f,g and leave $f_\mathrm{d}$ and $j$ as fitting parameters. We fit to measured amplitudes normalised as $\frac{A_{1,2}}{\max[A_{1,2}]}$, so only the fit value of $j$ has a physical meaning. The model of eq S16 describes the experiment well for $j = 1.72\times10^{13}$ Nm$^{-1}$kg$^{-1}$ with only a small amplitude excess in $A_2$ which likely originates from some higher-order nonlinear effect.

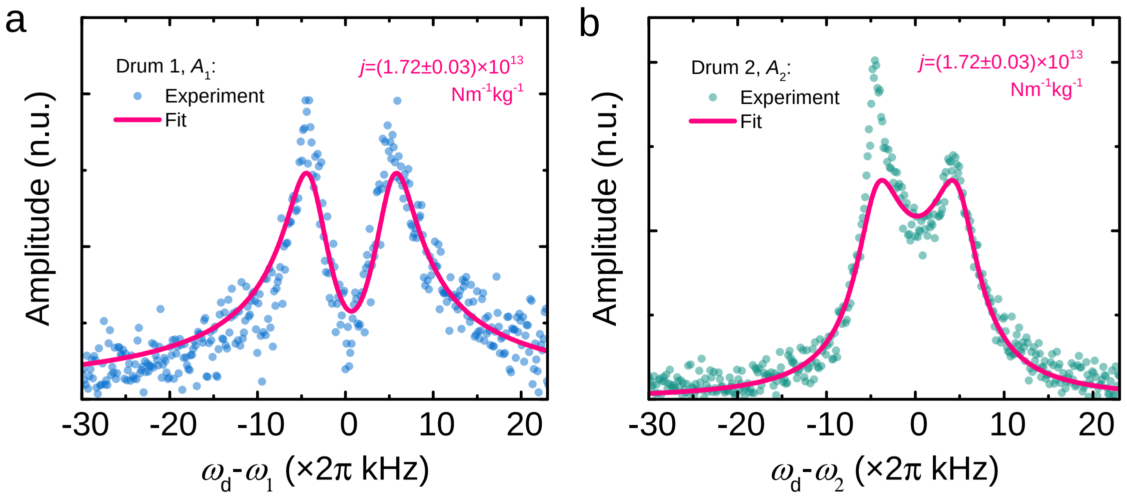


Figure S4: Amplitudes of a resonance frequency splitting $A_{1,2}$ for two drums (the same as in the main text Fig. 1 and 3.) at 4 K. (a,b) Filled dots - measured data, Solid lines - fit to the coupled oscillators model of eq S16.

# 4. Electromechanical coupling model

Suspended parts of a flake act as circular membrane capacitors $C_{1,2}$ together with the bottom gate electrodes of radius $r_{\rm g}$. The unsuspended region of the flake is situated on top of the grounded gold electrode. Ideally, if the material would be a good conductor, the DC resistance to grounded metal, $R_{\rm m}$, should drain all currents that are induced as a result of the motion. However, in the case of a poorly conducting material like $FePS_3$ and $MnPS_3$, the capacitance between flake and metal electrode can dominate the AC electrical coupling to ground, which mediates an electromechanical coupling between the membranes. We model this electrical coupling mechanism for $FePS_3$ and $MnPS_3$ by considering electrical equivalent DC and AC circuits of the membrane system, as shown in Fig. S5a. In doing so, we assume that the contact between the top gold electrode and the flake is ohmic for DC signals, such that the DC voltage established on the flake is $V_{\rm m,DC} \approx 0$ V, as shown in Fig. S5b. However, for the AC circuit shown in Fig. S5c, for which the AC impedance $\frac{1}{\omega_{\rm d} C_{\rm m}}$ is significantly lower than $R_{\rm m}$, $C_{\rm m}$ acts as a capacitive coupling element and produces an equivalent of a capacitive divider for the AC signal, that results in a time dependent voltage across both flakes (Fig. S5c).

As shown in Fig. S5, the time-varying capacitance $C_1(t)$ of the drum 1 and its time-dependent term $C_{1,\rm AC}(t)$ can be written as:

$$C_1(t) = \frac{\varepsilon_0\, \pi r_{\rm g}^2}{x_{\rm c} - x_1(t)} \approx \frac{\varepsilon_0\, \pi r_{\rm g}^2}{x_{\rm c}} \left(1 + \frac{x_1(t)}{x_{\rm c}}\right), \tag{S17}$$

$$C_{1,\rm AC}(t) = \frac{\varepsilon_0\, \pi r_{\rm g}^2}{x_{\rm c}^2} x_{10} \sin\left(\omega_{\rm d} t\right), \tag{S18}$$

where $x_{10}$ is the periodic displacement amplitude. We now consider the AC voltage between the flake and ground, $V_{\rm m,AC}$ and write the charge conservation equation of the system in Fig. S5c in the following form:

$$-\left(V_{\rm g,1} - V_{\rm m,AC}\right) C_{1,\rm AC}(t) + C_{\rm m} V_{\rm m,AC} = 0. \tag{S19}$$

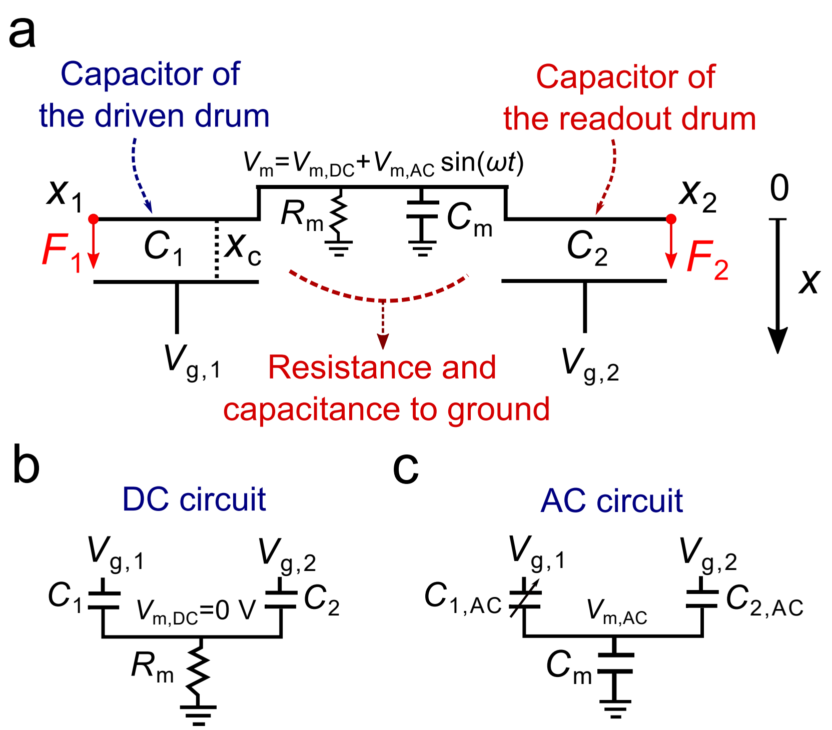


Figure S5: Schematic drawing of equivalent electrical circuit of two membrane capacitors. $V_{\mathrm{m}}$ is the voltage established between the membranes, $R_{\mathrm{m}}$ and $C_{\mathrm{m}}$, respectively, the resistance and capacitance between the ground electrode and the suspended flake, $F_{1,2}$ the force acting on the membrane, $C_{1,2}$ the capacitance between the membrane and bottom gate electrode separated by cavity distance $x_{\mathrm{c}}$.

To further simplify the derivation of corresponding forces acting on membranes, we use $C_{\mathrm{m}} >> C_{1,2}$ and that $x_1 >> x_2$ when driving the drum 1. Then, from the eq S19, $V_{\mathrm{m,AC}}$ becomes:

$$V_{\mathrm{m,AC}}(t) = \frac{V_{\mathrm{g,1}}\, C_{\mathrm{1,AC}}(t)}{C_{\mathrm{1,AC}}(t) + C_{\mathrm{m}}} \approx V_{\mathrm{g,1}} \frac{C_{\mathrm{1,AC}}(t)}{C_{\mathrm{m}}} \approx \frac{V_{\mathrm{g,1}}}{C_{\mathrm{m}}} \frac{\varepsilon_0\, \pi r_{\mathrm{g}}^2}{x_{\mathrm{c}}^2} x_{10} \sin\left(\omega_{\mathrm{d}} t\right). \tag{S20}$$

The voltage oscillation of $V_{\mathrm{m}}(\omega_{\mathrm{d}}, t)$ affects the potential between the membrane of drum 2 and its gate electrode and results in a oscillating force $F_2(t)$ acting on this membrane. This force can be described as:

$$F_2(t) = \frac{1}{2} \frac{\varepsilon_0\, \pi r_{\mathrm{g}}^2}{\left(x_{\mathrm{c}} - x_2(t)\right)^2} \left(V_{\mathrm{g,2}} - V_{\mathrm{m,AC}}\right)^2. \tag{S21}$$

Using that $V_{\mathrm{m,AC}} << V_{\mathrm{g},2}$ and $x_2 << x_{\mathrm{c}}$, this can be written as:

$$F_2(t) \approx \frac{1}{2}\frac{\varepsilon_0\,\pi r_{\mathrm{g}}^2}{x_{\mathrm{c}}^2}V_{\mathrm{g},2}^2 - \frac{\varepsilon_0\,\pi r_{\mathrm{g}}^2}{x_{\mathrm{c}}^2}V_{\mathrm{g},2}V_{\mathrm{m,AC}}(t). \tag{S22}$$

By substituting $V_{\mathrm{m,AC}}$ from eq S20 and taking only the time-dependent part of the eq S22, the force $F_{2,\mathrm{AC}}$ that drives the readout drum at $V_{\mathrm{g}} < 0$ V is:

$$F_{2,\mathrm{AC}}(t) = -\frac{\epsilon_0\,\pi r_{\mathrm{g}}^2}{x_{\mathrm{c}}^2}V_{\mathrm{g},2}V_{\mathrm{m,AC}}(t) \cong -\frac{\left(\varepsilon_0\,\pi r_{\mathrm{g}}^2\right)^2}{C_{\mathrm{m}}}\frac{V_{\mathrm{g},1}V_{\mathrm{g},2}}{x_{\mathrm{c}}^4}x_{10}\sin\left(\omega_{\mathrm{d}}t\right). \tag{S23}$$

However, at large $V_{\mathrm{g}}$ the membrane deflects down due to the introduced electrostatic force (see SI 1). The solution that accounts for the exact deflection shape would be rather complex.[1] However, one can substitute $x_{\mathrm{c}}$ in eq S23 for corresponding $x_{\mathrm{c}} - x_{\mathrm{g}}(V_{\mathrm{g}})$ for each membrane, under the assumption that the central part of the membrane is what contributes the most to the resultant change in $F_{2,\mathrm{AC}}$ due to deflection. This results in the final equation for the electrostatic force on drum 2, $F_{2,\mathrm{AC}}$, that is caused by the motion of drum 1 and its effect on the flake voltage $V_{\mathrm{m,AC}}$:

$$F_{2,\mathrm{AC}}(t) \cong -\left[\frac{\left(\epsilon_0\pi r_{\mathrm{g}}^2\right)^2}{C_{\mathrm{m}}}\frac{V_{\mathrm{g},1}\,V_{\mathrm{g},2}}{(x_{\mathrm{c}}-x_{\mathrm{g},1})^2\,(x_{\mathrm{c}}-x_{\mathrm{g},2})^2}\right]x_{10}\sin\left(\omega_{\mathrm{d}}t\right) = -J_{\mathrm{el}}x_{10}\sin\left(\omega_{\mathrm{d}}t\right), \tag{S24}$$

where $J_{\mathrm{el}}$ is the electrical coupling parameter from eq S11.

We now use eq S16 from SI 3, together with the coupling parameter $J \approx J_{\mathrm{el}}$ from eq S24 to calculate the amplitudes $A_{1,2}$ as a function of frequency, showing the resonance peak splitting. In Figure S6 we plot the measured data at 4 K fitted with eq S16, together with the model of eq S16 and S24 for $V_{\mathrm{g},1} = 37.21$ V, $V_{\mathrm{g},2} = 30$ V and $C_{\mathrm{m}} = 1.9$ pF. We use $\gamma_{1,2}(V_{\mathrm{g}})$ and $\omega_{1,2}(V_{\mathrm{g}})$ from the data in Fig. 1f,g and leave $f_{\mathrm{d}}$ in eq S16 as scaling factor. The $j = \frac{J}{\sqrt{m_1 m_2}} = 1.62\times10^{13}$ Nm$^{-1}$kg$^{-1}$, that we calculate using eq S24, describes the experiment well and is quantitatively close to $j = 1.72\times10^{13}$ Nm$^{-1}$kg$^{-1}$ that is extracted from the fit of the same experimental data to eq S16. This confirms that, even though quite simplified, our

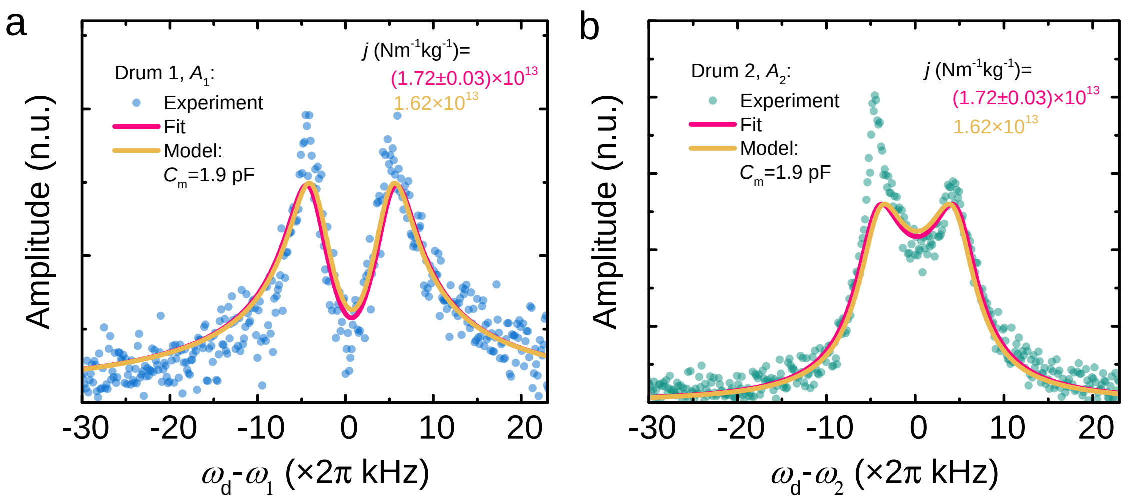


Figure S6: Normalized amplitudes of a resonance frequency splitting $A_{1,2}$ for two drums (the same as in the main text Fig. 1 and 3.) at 4 K. (a,b) Filled dots - measured data, Solid magenta lines - fit to the coupled oscillators model of eq S16 from Fig. S4, Solid orange lines - model of electrically coupled $FePS_3$ membranes described in SI 4 calculated using eq S16 and S24.

model explains the mechanism of strong coupling between distant membrane resonators.

# 5. Laser intensity and driving power dependence

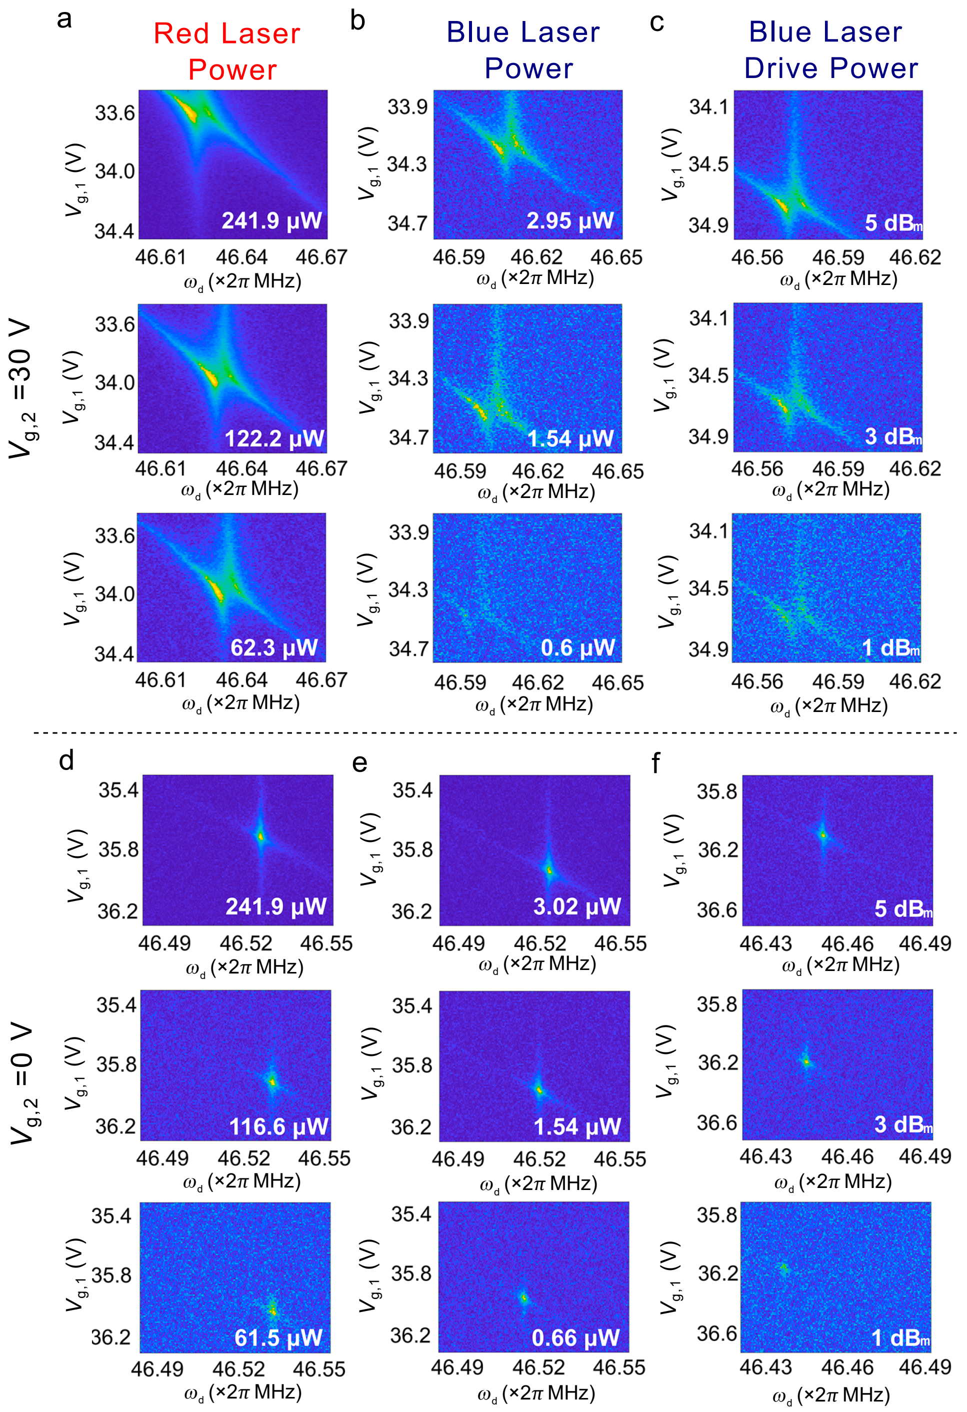


Figure S7: Normalized amplitudes of the resonance frequency splitting $A_2$ for different power and drive of lasers at $T = 4$ K. (a-c) Measured $A_2$ at $V_{g,2} = 30$ V. (d-f) Measured $A_2$ at $V_{g,2} = 0$ V. Respective laser power or drive power is labeled in all panels. (a), (d), (c) and (f) is measured at $P_{\text{blue}} \approx 1.5\ \mu$W. (b), (e), (c) and (f) is measured at $P_{\text{red}} \approx 100\ \mu$W. (a), (b), (d) and (e) is measured at $P_{\text{d}} \approx 5$ dBm. Within all figures of top and bottom panels no substantial change in the splitting $2g$ was observed.

# 6. Laser position dependence

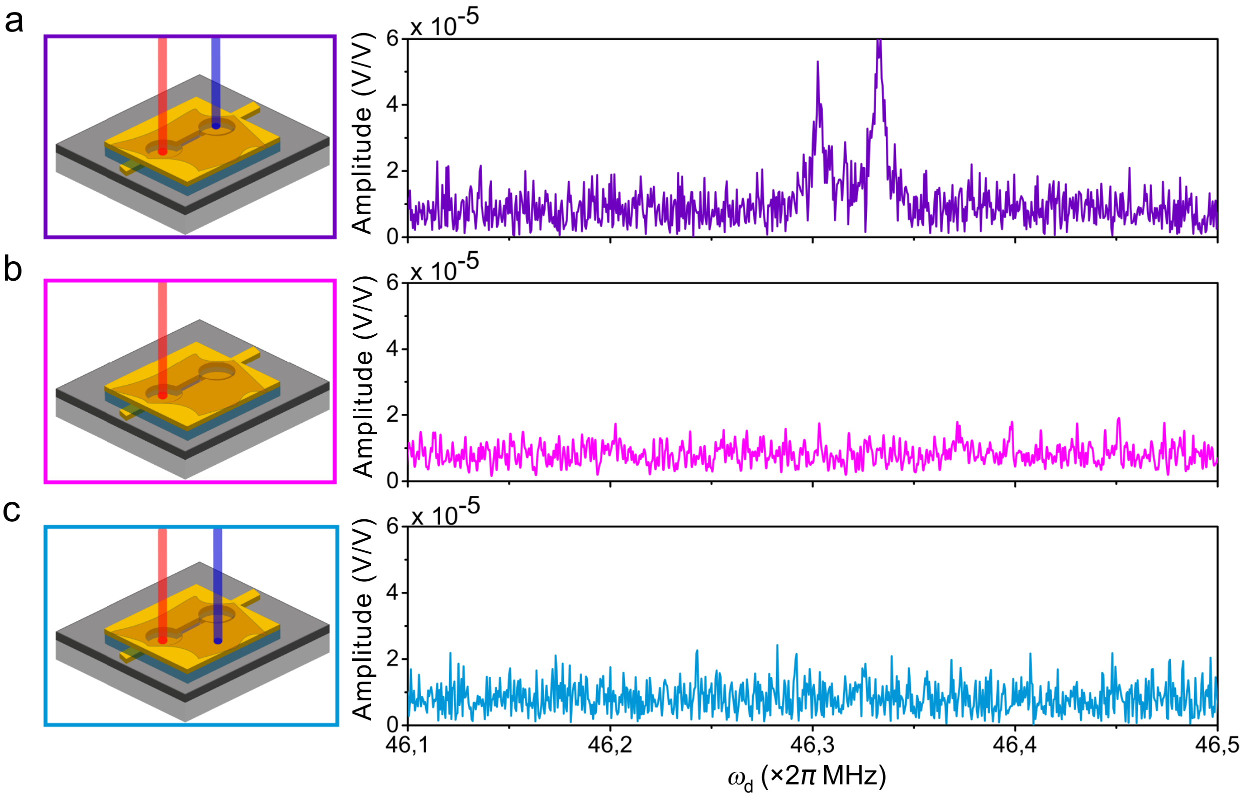


Figure S8: Measured amplitudes of the resonance frequency splitting $A_2$ at blue laser drive power $P_\mathrm{d} = 1$ dBm and 4 K. Blue laser is optothermally actuating the motion of the drum which in turn through electrical coupling (described in SI 3 and 4) put the other drum in motion, that is probed by the red laser. (a-c) Left panels: Schematics of the laser position. Right panel: measured resonance peak splitting or its absence at respective laser position.

# 7. Test sample without a micro-channel connecting two suspended drums

It is important to check the possible contribution of other tension-related coupling effects in our experiments. Also, an informative test is required for understanding if the ground capacitor $C_\mathrm{m}$ described in SI 4 is possibly formed because of the non-grounded part of the flake that is suspended over the channel connecting two circular membranes. To do so, we fabricate an additional test sample without this channel, now having a top ground electrode

electrically grounding the area between suspended drums, mechanically supported as shown in Fig. S9a.

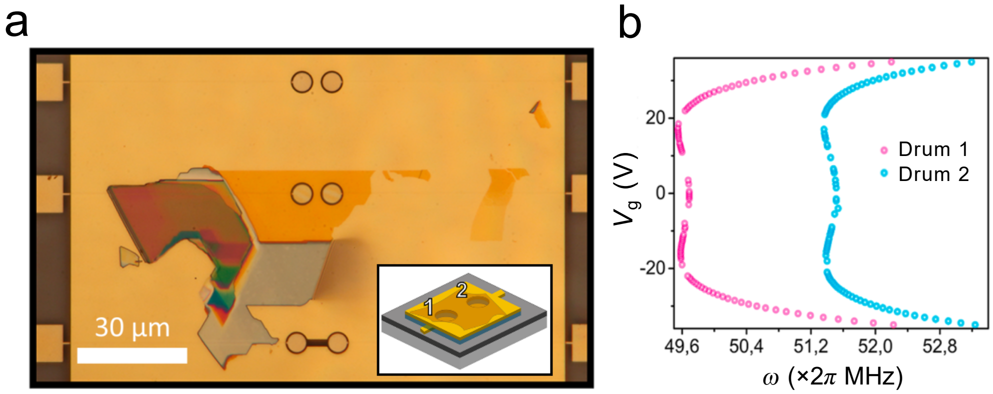


Figure S9: Sample of $14.5 \pm 0.3$ nm thin $FePS_3$ without a channel connecting the two membranes. (a) Optical image of the sample. Inset: Schematics of the sample. Cavity depth $x_c = 220$ nm, drum radius $r = 3$ $\mu$m, bottom gate electrode radius $r_g = 2.5$ $\mu$m. (b) Frequency $\omega(V_g)$ of the resonance peaks for the two drums (the same as in the main text Fig. 2d) at 4 K.

Following the methodology from SI 1 and the one described in the main text, we measure $\omega(V_g)$ for each membrane and plot it in Fig. S9b. Although $\omega_2$ is notably larger than $\omega_1$ at $V_g = 0$ V, we are able to match these frequencies to establish $\omega_1 = \omega_2$ condition with non-zero $V_{g,1}$ and $V_{g,2}$. We now sweep $V_{g,2}$ from 0 to 32 V and measure the amplitude $A_2$ of the avoided crossing by driving drum 1 and measuring drum 2, as shown in Fig. S10. The splitting of the resonance peak occurs only at large $V_{g,2}$ with a $2g$ value similar to the case described in Fig. 2 and 3. Thus, other effects arising due to the channel connecting the drums, like tension- or phonon-mediated coupling as well as its effect on $C_m$, do not contribute significantly to the coupling mechanism and thus can be neglected.

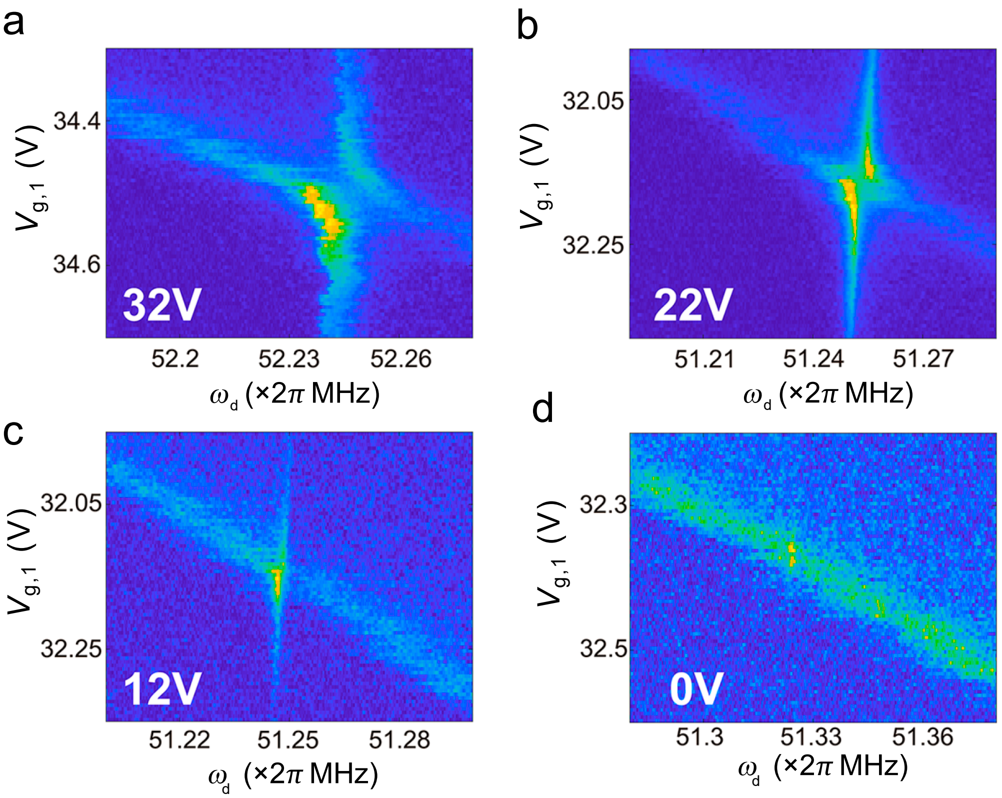


Figure S10: Normalized amplitudes of the resonance frequency splitting $A_2$ for two drums from Fig. S9 at 4 K. $V_{g,2}$ is labeled in all panels.

# References


(1) Chen, C. *Graphene NanoElectroMechanical Resonators and Oscillators*; Ph.D. thesis, Columbia University, 2013.

(2) Landau, L. D.; Lifshitz, E. M. *Theory of Elasticity*, 3rd ed.; Elsevier, 1986.

(3) Timoshenko, S. P. *Theory of Plates and Shells*, 2nd ed.; McGraw Hill: New York, 1959.

(4) Šiškins, M.; Lee, M.; Mañas-Valero, S.; Coronado, E.; Blanter, Y. M.; van der Zant, H. S. J.; Steeneken, P. G. Magnetic and Electronic Phase Transitions Probed by Nanomechanical Resonators. *Nat. Commun.* **2020**, *11*, 2698.

(5) Hashemi, A.; Komsa, H.-P.; Puska, M.; Krasheninnikov, A. V. Vibrational Properties of

Metal Phosphorus Trichalcogenides from First-Principles Calculations. *J. Phys. Chem. C* **2017**, *121*, 27207–27217.

(6) Weber, P.; Güttinger, J.; Tsioutsios, I.; Chang, D. E.; Bachtold, A. Coupling Graphene Mechanical Resonators to Superconducting Microwave Cavities. *Nano Lett.* **2014**, *14*, 2854–2860.

(7) Castellanos-Gomez, A.; Singh, V.; van der Zant, H. S. J.; Steele, G. A. Mechanics of Freely-Suspended Ultrathin Layered Materials. *Ann. Phys. (Berl.)* **2014**, *527*, 27–44.

(8) Will, M.; Hamer, M.; Müller, M.; Noury, A.; Weber, P.; Bachtold, A.; Gorbachev, R. V.; Stampfer, C.; Güttinger, J. High Quality Factor Graphene-Based Two-Dimensional Heterostructure Mechanical Resonator. *Nano Lett.* **2017**, *17*, 5950–5955.

(9) Song, X.; Oksanen, M.; Sillanpää, M. A.; Craighead, H. G.; Parpia, J. M.; Hakonen, P. J. Stamp Transferred Suspended Graphene Mechanical Resonators for Radio Frequency Electrical Readout. *Nano Lett.* **2011**, *12*, 198–202.

(10) Zanette, D. H. Energy Exchange Between Coupled Mechanical Oscillators: Linear Regimes. *J. Phys. Commun.* **2018**, *2*, 095015.
